# Supplementary material for: Nanoscale sheared droplet: Volume-of-Fluid, phase-field and no-slip molecular dynamics
Source: arXiv:2112.09682 ancillary file (2022-04-12)
Supplement: Supplementary file 1 [file supMat.pdf]

*Supplementary online material for “Nanoscale sheared droplet: Volume-of-Fluid, phase-field and no-slip molecular dynamics”*

Uģis Lācis, Michele Pellegrino, Johan Sundin, Berk Hess, Gustav Amberg, Stéphane Zaleski & Shervin Bagheri

Supplementary File 1: Data files and plotting scripts to reproduce simulation based curves in the main paper. The files are grouped according to figure number, see included README file. Archive file name “FigureData.tar.gz”.

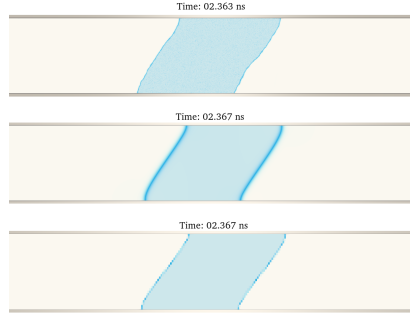

Supplementary Movie 1: Comparison between MD simulation (top part), PF simulation (center part) and VOF simulation (bottom part) at  $\theta_0 = 95^\circ$  and  $Ca = 0.30$ . Time instant is shown above each simulation. Movie file name “supMov1\_MD\_PF\_VOF\_ca95\_Ca0.30.mp4”.

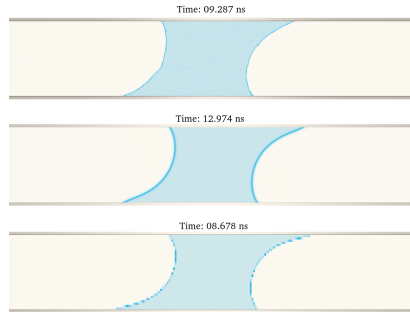

Supplementary Movie 2: Comparison between MD simulation (top part), PF simulation (center part) and VOF simulation (bottom part) at  $\theta_0 = 38^\circ$  and  $Ca = 0.05$ . Time instant is shown above each simulation. Movie file name “supMov2\_MD\_PF\_VOF\_ca38\_Ca0.05.mp4”.

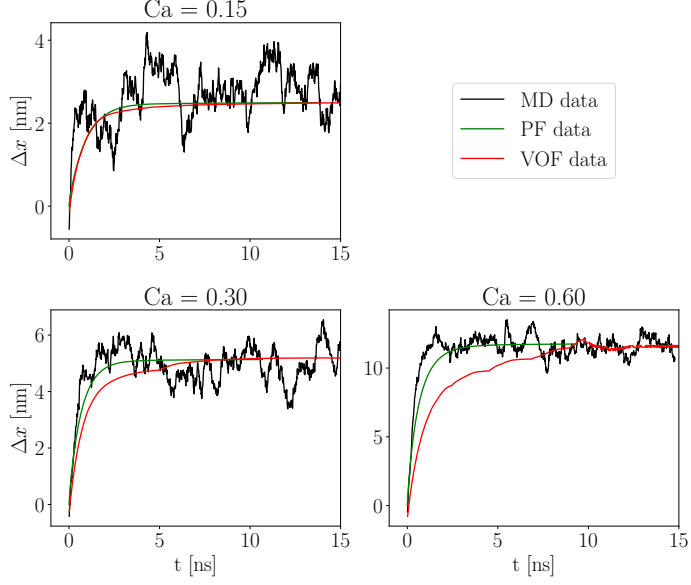

Supplementary Figure 1: Time evolution of  $\Delta x$  in MD, PF and VOF for  $Ca \in (0.15, 0.60)$ . Equilibrium contact angle  $\theta_0 = 127^\circ$ .

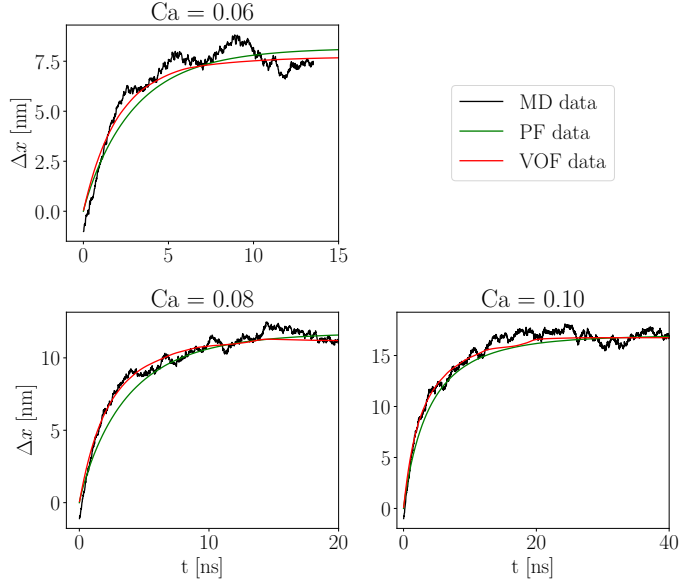

Supplementary Figure 2: Time evolution of  $\Delta x$  in MD, PF and VOF for  $Ca \in (0.06, 0.10)$ . Equilibrium contact angle  $\theta_0 = 69^\circ$ .

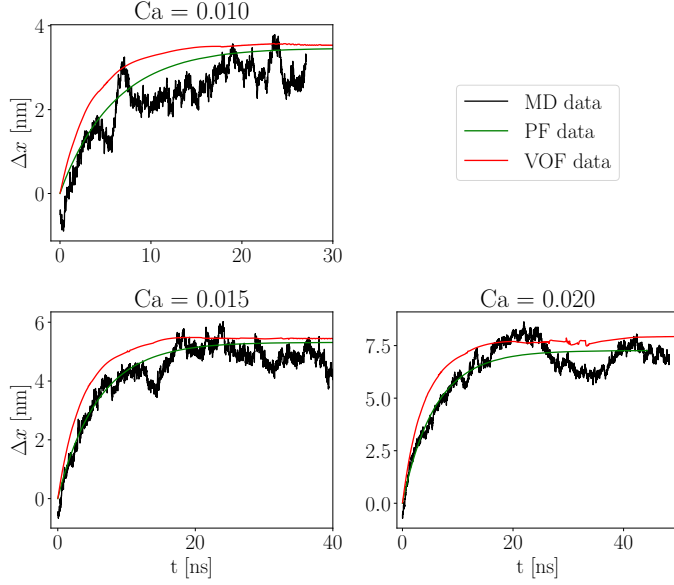

Supplementary Figure 3: Time evolution of  $\Delta x$  in MD, PF and VOF for  $Ca \in (0.01, 0.02)$ . Equilibrium contact angle  $\theta_0 = 38^\circ$ .

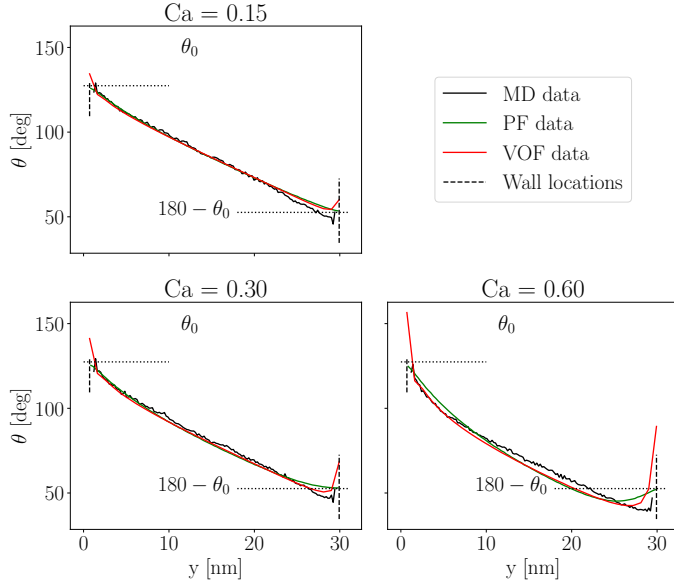

Supplementary Figure 4: Comparison between interface shape of MD, PF and VOF for all steady  $Ca$  numbers of  $\theta_0 = 127^\circ$  configuration. Equilibrium angles and solid wall locations are shown with black dotted and dashed lines, respectively.

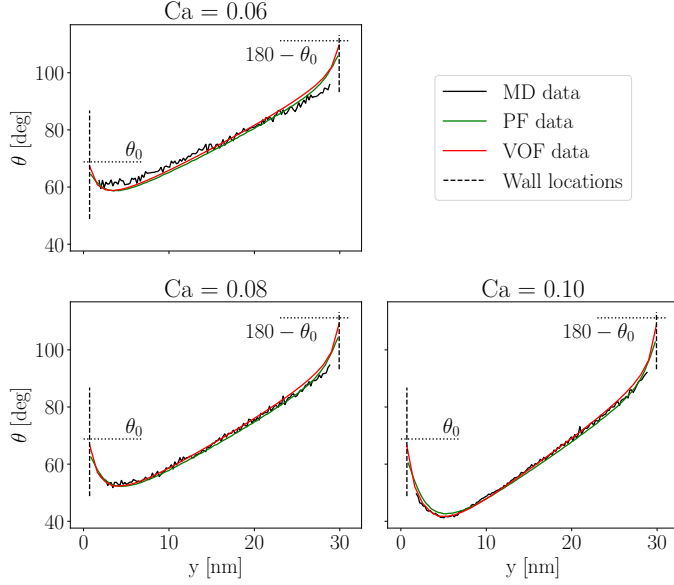

Supplementary Figure 5: Comparison between interface shape of MD, PF and VOF for all steady  $Ca$  numbers of  $\theta_0 = 69^\circ$  configuration. Equilibrium angles and solid wall locations are shown with black dotted and dashed lines, respectively.

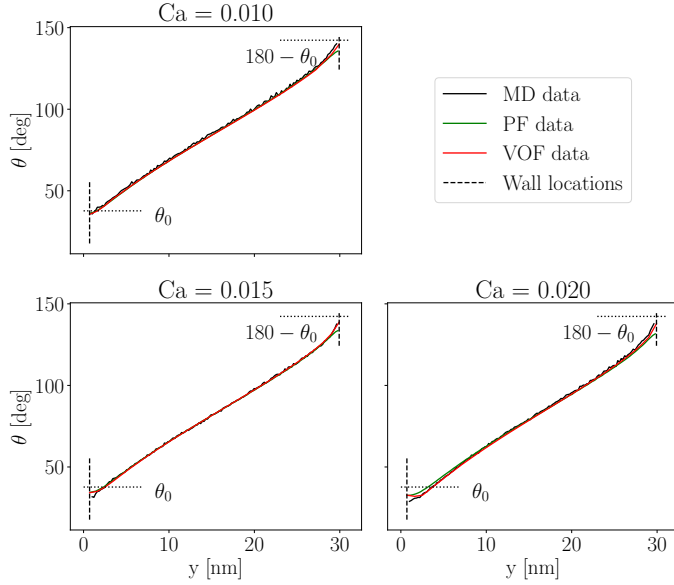

Supplementary Figure 6: Comparison between interface shape of MD, PF and VOF for all steady  $Ca$  numbers of  $\theta_0 = 38^\circ$  configuration. Equilibrium angles and solid wall locations are shown with black dotted and dashed lines, respectively.

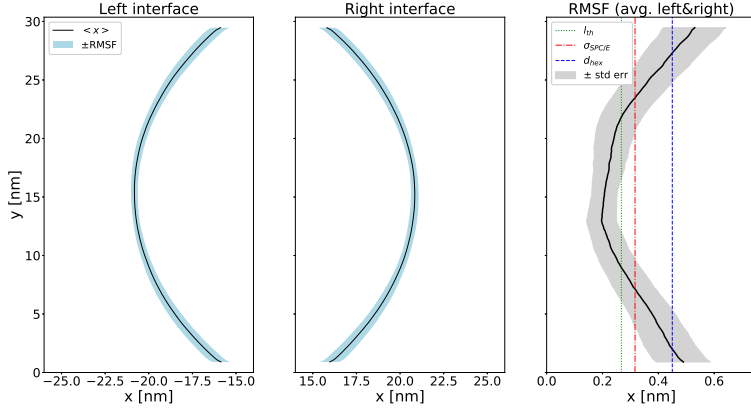

Supplementary Figure 7: Equilibrium average interface profile  $\langle x(y) \rangle$  and root-mean-square fluctuation  $\sqrt{\langle x^2(y) \rangle - \langle x(y) \rangle^2}$  for  $\theta_0 = 127^\circ$ , computed by averaging frames over a time window of 16.25 nanoseconds.

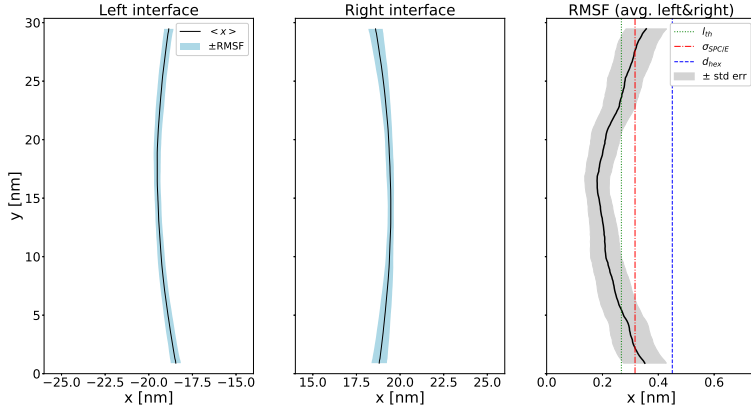

Supplementary Figure 8: Equilibrium average interface profile  $\langle x(y) \rangle$  and root-mean-square fluctuation  $\sqrt{\langle x^2(y) \rangle - \langle x(y) \rangle^2}$  for  $\theta_0 = 95^\circ$ , computed by averaging frames over a time window of 13.75 nanoseconds.

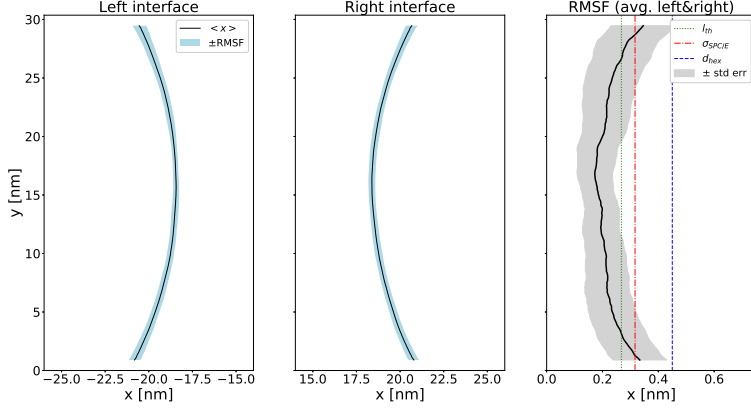

Supplementary Figure 9: Equilibrium average interface profile  $\langle x(y) \rangle$  and root-mean-square fluctuation  $\sqrt{\langle x^2(y) \rangle - \langle x(y) \rangle^2}$  for  $\theta_0 = 69^\circ$ , computed by averaging frames over a time window of 6.25 nanoseconds.

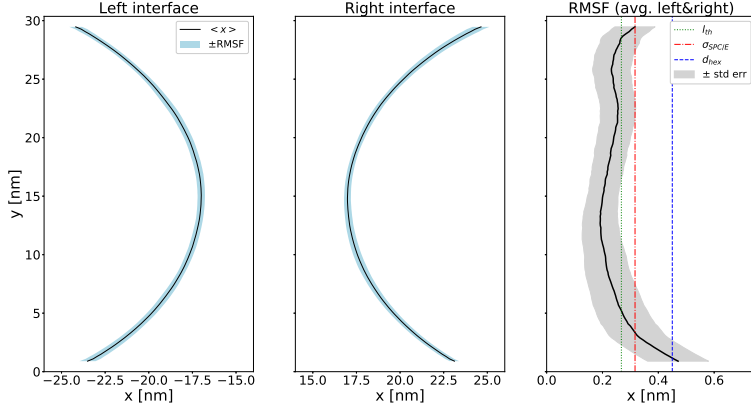

Supplementary Figure 10: Equilibrium average interface profile  $\langle x(y) \rangle$  and root-mean-square fluctuation  $\sqrt{\langle x^2(y) \rangle - \langle x(y) \rangle^2}$  for  $\theta_0 = 38^\circ$ , computed by averaging frames over a time window of 10.0 nanoseconds.
